# Supplementary material for: Quantum Rate-Distortion Coding of Relevant Information
Source: arXiv:1704.02903 ancillary file (2019-02-05)
Supplement: Supplementary file 1 [file randomchannels.pdf]

# Quantum Rate Distortion Coding for the Relevant Information

## Supplementary Material

This worksheet contains the random search optimisation algorithm that is used for finding the communication rate  $\hat{R}(J)$  numerically.

The algorithm works as follows. A channel  $N$  is constructed from a collection of up to  $n$  Krauss matrices, using the standard formula  $N(\rho) = \sum_{i=1}^n K_i \rho K_i^*$  for a given density matrix  $\rho$ . Here the  $K_i$  are 2x2 randomly generated matrices with entries given by complex numbers in a certain interval, which we normalize as appropriate. Given a channel and an input state (the density matrix  $\rho_{xy}$ , given here by a 4 x 4 matrix, the code computes the corresponding values of the "information ratios"

$J = \frac{I(\tilde{X}; Y)}{I(X; Y)}$  and  $\hat{R} = \frac{I(X; \tilde{X})}{I(X; X)}$  (although in the code it is called  $M$  at places). Then, it checks whether the value of  $\hat{R}(J)$  obtained is lower than any of the previously recorded values for the corresponding  $J$ . In case it is, the list of minimal values ( $\text{minf}$ ) will be updated using this channel. Based on this list, we also select the next channels to use in the algorithm in search of a new optimal channel. That is, we compute new channels by taking (recursively) random variations using a Gaussian distribution of a previously computed list of channels with minimal "information ratio"  $\hat{R}$ .

After trying variations of every channel in the list, this procedure terminates when the number of updates in the list will become irrelevant compared to the total number of channels, namely when the list no longer changes significantly. We then plot a graph that visualizes the list of minimal values of  $\hat{R}$  found with the routines above. Specifically, it plots an approximation to the curve  $\hat{R}(J)$ .

### randomChannel()

Creates a randomly chosen channel, with up to  $n$  Krauss matrices.

Parameters:  $n$  - the maximum number of Krauss operators to use (must be  $\geq 2$ )

Return value: The channel (represented by its Krauss operators)

```
> randomChannel:=proc(n)
  local i,nn,krauss,sum,adj;
  nn:=RandomTools[Generate](integer(range=2..n));
  krauss:=Array(1..nn);
  sum:=Matrix(2,2);
  for i from 1 to nn do
```

```

    krauss[i]:=RandomTools[Generate]('Matrix'(complex(float
(method = uniform, range=-1..1)),2,2));
    sum := sum + krauss[i].(krauss[i]^*);
end;
adj:=LinearAlgebra[MatrixFunction](sum,1/sqrt(x),x);
for i from 1 to nn do
    krauss[i] := adj.krauss[i];
end;
return krauss;
end;

```

### **randomChannelVariation()**

Produces a random variation of a given channel, by modifying each matrix entry of the Krauss operators by a Gaussian random variable (and then normalizing)

Parameters: ch - the channel to be varied

sigma - the variance of the Gaussian distribution (its mean value will always be 0)

Return value: the channel after random variation

```

> randomChannelVariation:=proc(ch,sigma)
    local krauss,n,i,sum,adj;
    n := ArrayTools[Size](ch, 2);
    krauss:=Array(1..n);
    sum:=Matrix(2,2);
    for i from 1 to n do
        krauss[i] := ch[i] + RandomTools[Generate]('Matrix'(complex
(distribution(Normal(0,sigma))),2,2));
        sum := sum + krauss[i].(krauss[i]^*);
    end;
    adj:=LinearAlgebra[MatrixFunction](sum,1/sqrt(x),x);
    for i from 1 to n do
        krauss[i] := adj.krauss[i];
    end;
    return krauss;
end;

```

### **elevate1()**

Given a 2x2 matrix A, compute the 4x4 matrix  $\mathbf{1} \otimes A$ .

Parameters: a - the 2x2 input matrix

Return value -  $\mathbf{1} \otimes A$

```

> elevate1:=proc(a)
    local b;
    b:=Matrix(4,4);
    b[1,1]:=a[1,1];
    b[1,2]:=a[1,2];
    b[2,1]:=a[2,1];
    b[2,2]:=a[2,2];
    b[3,3]:=a[1,1];

```

```

    b[3,4]:=a[1,2];
    b[4,3]:=a[2,1];
    b[4,4]:=a[2,2];
    return b;

```

**end proc;**

**elevate2()**

Given a 2x2 matrix A, compute the 4x4 matrix  $A \otimes \mathbf{1}$ .

Parameters: a - the 2x2 input matrix

Return value -  $A \otimes \mathbf{1}$

**> elevate2:=proc(a)**

```

    local b;
    b:=Matrix(4,4);
    b[1,1]:=a[1,1];
    b[2,2]:=a[1,1];
    b[1,3]:=a[1,2];
    b[2,4]:=a[1,2];
    b[3,1]:=a[2,1];
    b[4,2]:=a[2,1];
    b[3,3]:=a[2,2];
    b[4,4]:=a[2,2];
    return b;

```

**end proc;**

**ptrace1()**

Computes the partial trace over the first component of the tensor product.

Parameters: b - a 4x4 matrix

Return value:  $tr_1 b$  as a 2x2 matrix

**> ptrace1:=proc(b)**

```

    local a;
    a:=Matrix(2,2);
    a[1,1]:=b[1,1]+b[3,3];
    a[1,2]:=b[1,2]+b[3,4];
    a[2,1]:=b[2,1]+b[4,3];
    a[2,2]:=b[2,2]+b[4,4];
    return a;

```

**end proc;**

**ptrace2()**

Computes the partial trace over the second component of the tensor product.

Parameters: b - a 4x4 matrix

Return value:  $tr_2 b$  as a 2x2 matrix

**> ptrace2:=proc(b)**

```

    local a;
    a:=Matrix(2,2);
    a[1,1]:=b[1,1]+b[2,2];

```

```

    a[1,2]:=b[1,3]+b[2,4];
    a[2,1]:=b[3,1]+b[4,2];
    a[2,2]:=b[3,3]+b[4,4];
    return a;
end proc;

```

### **applyChannel()**

Apply a channel in the second part of the tensor product to a state; that is, if  $N$  is the channel in question, then compute  $(id \otimes N)(A)$  where  $A$  is a state matrix on the 4-dimensional tensor product state.

Parameters: a - the input state (a 4x4 matrix)

ch - the channel  $N$  to be applied (represented by Krauss operators)

Return value: the output state (a 4x4 matrix)

```

> applyChannel:=proc(a,ch)
    local ac,i,n,ue;
    ac := Matrix(4,4);
    n := ArrayTools[Size](ch, 2);
    for i from 1 to n do
        ue := elevate1(ch[i]);
        ac := ac + (ue^*.a.ue);
    end;

    return ac;
end;

```

### **entropy()**

Compute the entropy of a state, given by a general square matrix.

Parameters: a - the state matrix (assumed to be positive and normalized)

Return value: the entropy, i.e., the number  $-\text{tr}(a \ln a)$ .

```

> entropy:=proc(a)
    local ev,rev,iev,i,sum;
    ev:=LinearAlgebra[Eigenvalues](a);
    sum :=0.0;
    for i from 1 to LinearAlgebra[RowDimension](a) do
        rev:=Re(ev[i]);iev:=Im(ev[i]);
        if rev < -1e-7 or rev > 1 + 1e-7 or abs(iev) > 1e-7 then
            error("unexpected eigenvalue: %1", ev[i]);
        elif rev > 0.0000001 then
            sum := sum - rev*log(rev);
        end;
    end;
    return sum;
end;

```

### **mutualInf()**

Compute the mutual information of a state on the tensor product space.

Parameters: b - a state matrix (4x4)

Return value: the mutual information  $I(X,Y)$  in that state.

```
> mutualInf:=proc(b)  
  local b1,b2;  
  b1:=ptrace1(b);  
  b2:=ptrace2(b);  
  return entropy(b1)+entropy(b2)-entropy(b);  
end;
```

**infoRatio()**

Given a channel, an input state and its purification, compute the ratios  $J = I(X\sim,Y)/I(X,Y)$  and  $M := I(X\sim,X)/I(X,X')$ .

Parameters: s - a list of the input state (s[1]) on XY and its purification on XX'. States are given as their 4x4 density matrices.

ch - the channel to be applied.

Return value: [J,M] with J and M defined as above.

```
> infoRatio:=proc(s,ch)  
  local pures,inputs,purech,inputch,J,M;  
  inputs:=s[1];pures:=s[2];  
  inputch:=applyChannel(inputs,ch);  
  purech:=applyChannel(pures,ch);  
  J:= mutualInf(inputch)/mutualInf(inputs);  
  M:= mutualInf(purech)/mutualInf(pures);  
  return [J,M];  
end;
```

**purify()**

Compute purification (on XX') of an input state (on XY).

Parameters: s - the density matrix (4x4) of the input state

Return value: the density matrix (4x4) of its purification.

```
> purify:=proc(s)  
  local s2,e,v,i,j,ei,ej,mij,p;  
  s2:=ptrace1(s);  
  v,e := LinearAlgebra[Eigenvectors](s2);  
  p := Matrix(4,4);  
  for i from 1 to 2 do  
    for j from 1 to 2 do  
      ei := e[1..2,i];  
      ej := e[1..2,j];  
      mij := elevate1(ei.ej^*).elevate2(ei.ej^*);  
      p := p + sqrt(v[i]*v[j]) * mij;  
    end;  
  end;  
  return p;  
end;
```

**tryChannel()**

Given a channel and an input state, compute the corresponding "information ratios"

(J and M) and check whether M is lower than any of the previously recorded values for the corresponding J.

Parameters: s - the input state and its purification

ch - the channel to be applied

inflist - a list of previously found minimal values for M, indexed J on a discrete scale

Return value: whether the list of minimal values has been updated using this channel (true or false)

```
> tryChannel:=proc(s,ch,inflist)  
  local cnt,ratio,n,used,jidx,k;  
  
  ratio:=infoRatio(s,ch);  
  
  used := false;  
  n := ArrayTools[Size](inflist,2);  
  jidx:=min(floor(n*ratio[1]), ArrayTools[Size](inflist,2) - 1);  
  if inflist[jidx][1]>ratio[2]+1e-6 then  
    used :=true;  
    for k from 0 to jidx do  
      if inflist[k][1] > ratio[2] then  
        inflist[k][1]:=ratio[2];  
        inflist[k][2]:=ch;  
      end;  
    end;  
  end;  
  return used;
```

**end;**

**varyChannelRecursive()**

Given a channel and an input state, take a number of random variations of the channel and try whether these give lower values for the "information ratio" M than the previously known ones. If any of these turn out to yield lower values of M, random variations are then applied to these new channels recursively.

Parameters: s - the input state and its purification

ch - the channel to be applied

inflist - a list of previously found minimal values for M, indexed J on a discrete scale

sigma - standard deviation used for the random variation

depth - number of attempts for randomly varying the channel

Return value: whether the list of minimal values has been updated using the randomly varied channels (true or false)

```
> varyChannelRecursive:=proc(s,ch,inflist,sigma,depth)  
  local used, someused, i, ch2;  
  someused:=false;
```

```

    for i from 1 to depth do
        ch2:=randomChannelVariation(ch,sigma);
        used:=tryChannel(s,ch2,inflist);
        if used then
            varyChannelRecursive(s,ch2,inflist,sigma,depth);
            someused:=true;
        end;
    end;
    return someused;
end;

```

#### **addSamples()**

Given an input state, choose a number of channels at random and see whether these give lower values for the "information ratio"  $M$  than the previously known ones. No recursion is used.

Parameters:  $s$  - the input state and its purification

$n$  - number of random channels to try

$inflist$  - a list of previously found minimal values for  $M$ , indexed  $J$  on a discrete scale

Return value: none

```

> addSamples:=proc(s,n,inflist)
    local i, ch;
    for i from 1 to n do
        ch:=randomChannel(4);
        tryChannel(s,ch,inflist);
    end;
end;

```

#### **refine()**

Starting from a previously computed list of channels with minimal "information ratio"  $M$ , compute random variations of each of these (recursively), in search of a new optimal channel. After trying variations of every channel in the list, the procedure then computes how many channels in the start list have actually, after variation, lead to a change in the of optimal channels. The process is repeated until the ratio of "changed" channels and total number of channels falls below a given value, i.e., until the list no longer changes significantly.

Parameters:  $s$  - the input state and its purification

$\sigma$  - standard deviation used for the random variation

$depth$  - number of random variations to take of every channel

$threshold$  - the process will repeat until the ratio "changed channels" vs "total channels" falls below this value.

$inflist$  - a list of previously found minimal values for  $M$ , indexed  $J$  on a discrete scale

Return value: none

```

> refine:=proc(s,sigma,depth,threshold,inflist)
    local i, nticks, ch, updatedTicks, used;

```

```

nticks := ArrayTools[Size](inflist,2);
updatedTicks := nticks;
while updatedTicks > threshold*nticks do
  updatedTicks := 0;
  for i from 0 to nticks-1 do
    if inflist[i][1] < 1 then
      ch := inflist[i][2];
      used := varyChannelRecursive(s,ch,inflist,sigma,depth);
      if used then
        updatedTicks := updatedTicks + 1;
      end;
    end;
  end;
  printf("One round of refinement with sigma=%f, depth=%d;
change rate: %f \n", sigma, depth, updatedTicks/nticks);
end;
end;

```

### plotResult()

Plots a graph that visualizes the list of minimal values of M found with the routines above. That is, it plots an approximation to the curve for M(J).

Parameters: inflist - a list of previously found minimal values for M, indexed J on a discrete scale

Return value: none

```

> plotResult:=proc(inflist)
  local pp,bp,lp,minfp,nticks,i,rhatlabel;
  nticks:=ArrayTools[Size](inflist,2);
  lp:=[plot(x/2,x=0..1,color=blue),plot(x,x=0..1,color=blue)];
  minfp:=Array(1..nticks);
  for i from 0 to nticks-1 do minfp[i+1]:=[(i/nticks),inflist[i]
[1]] end;
  bp:=plots[pointplot](minfp,connect=true,color=red);
  rhatlabel:="#mover(mi("R"),mi("^"))^(J);
  plots[display](lp,bp,gridlines=true,labels=["J",rhatlabel]);
end;

```

The following functions generate examples of input states. They all return a list with two entries: s[1] is the input state on XY and s[2] is a corresponding purifies state on XX'. Both of these are represented as 4x4 density matrices.

### stateExample1()

Returns a "classical" state, i.e., a state without entanglement between x and y.

Namely, given nonnegative numbers  $p_1, p_2, p_3, p_4$ , the state with the density matrix

$$\rho_{YX} = p_1 \begin{vmatrix} \uparrow\uparrow \\ \downarrow\downarrow \end{vmatrix} + p_2 \begin{vmatrix} \uparrow\downarrow \\ \downarrow\uparrow \end{vmatrix} + p_3 \begin{vmatrix} \downarrow\uparrow \\ \uparrow\downarrow \end{vmatrix} + p_4 \begin{vmatrix} \downarrow\downarrow \\ \uparrow\uparrow \end{vmatrix}$$

It is assumed here that  $p_1 + p_2 + p_3 + p_4 = 1$ .

Parameters: p1, p2, p3, p4 - the parameters  $p_j$  above.

Return value: the density matrix of the state and of a purification

```
> stateExample1:=proc(p1,p2,p3,p4)
  local purestate1,purestate2,purestate3,purestate4,redstate,
  purevec,purevec1,purevec2,purestate,inputstate;
  purestate1:=Matrix([[1,0,0,0],[0,0,0,0],[0,0,0,0],[0,0,0,0]]);
  purestate2:=Matrix([[0,0,0,0],[0,1,0,0],[0,0,0,0],[0,0,0,0]]);
  purestate3:=Matrix([[0,0,0,0],[0,0,0,0],[0,0,1,0],[0,0,0,0]]);
  purestate4:=Matrix([[0,0,0,0],[0,0,0,0],[0,0,0,0],[0,0,0,1]]);
  inputstate:= p1*purestate1+p2*purestate2+p3*purestate3+p4*
  purestate4;
  redstate:=ptrace1(inputstate);
  purevec1:= Vector([1,0,0,0]);
  purevec2:=Vector([0,0,0,1]);
  purevec:=sqrt(redstate[1,1])*purevec1+sqrt(redstate[2,2])*
  purevec2;
  purestate:=purevec.LinearAlgebra[Transpose](purevec);
  return [inputstate,purestate];
end;
```

**stateExample2()**

Returns a state with entanglement, namely,

$$\rho_{YX} = 0.5 \begin{vmatrix} \uparrow\uparrow \\ \downarrow\downarrow \end{vmatrix} \begin{vmatrix} \uparrow\uparrow \\ \downarrow\downarrow \end{vmatrix} + 0.25 \begin{vmatrix} \uparrow\uparrow \\ \downarrow\downarrow \end{vmatrix} \begin{vmatrix} \uparrow\downarrow \\ \downarrow\uparrow \end{vmatrix} + 0.25 \begin{vmatrix} \uparrow\downarrow \\ \downarrow\uparrow \end{vmatrix} \begin{vmatrix} \uparrow\uparrow \\ \downarrow\downarrow \end{vmatrix} + 0.5 \begin{vmatrix} \uparrow\downarrow \\ \downarrow\uparrow \end{vmatrix} \begin{vmatrix} \uparrow\downarrow \\ \downarrow\uparrow \end{vmatrix}.$$

Parameters: none

Return value: the density matrix of the state and of a purification

```
> stateExample2:=proc()
  local purestate1,purestate2,purestate3,purestate4,redstate,
  purevec,purevec1,purevec2,purestate,inputstate;
  inputstate:=Matrix([[0.5,0,0,0.25],[0,0,0,0],[0,0,0,0],[0.25,0,
  0,0.5]]);
  purestate:=purify(inputstate);
  return [inputstate,purestate];
end;
```

**stateExample3()**

$$\rho_{YX} = a \begin{vmatrix} v \\ w \end{vmatrix} \begin{vmatrix} v \\ w \end{vmatrix} + b \begin{vmatrix} v \\ w \end{vmatrix} \begin{vmatrix} w \\ v \end{vmatrix} + b \begin{vmatrix} w \\ v \end{vmatrix} \begin{vmatrix} v \\ w \end{vmatrix} + a \begin{vmatrix} w \\ v \end{vmatrix} \begin{vmatrix} w \\ v \end{vmatrix}$$

with the normalized vectors

$$v = \frac{1}{\sqrt{2}} (|\uparrow\uparrow\rangle + |\downarrow\downarrow\rangle), \quad w = \frac{1}{\sqrt{2}} (|\uparrow\downarrow\rangle - |\downarrow\uparrow\rangle).$$

Parameters: a,b - constants as described above

Return value: the density matrix of the state and of a purification

```
> stateExample3:=proc(a,b)
  local purevec1,purevec2,purestate,inputstate;
  purevec1:=evalf(Vector([1/sqrt(2),0,0,1/sqrt(2)]));
```

```

    purevec2:= Vector([0,0,0,1]);
    inputstate:= a*(purevec1.purevec1^*) + b*(purevec2.purevec2^*);
    purestate:=purify(inputstate);
    return [inputstate,purestate];
end;

```

The following is an example of a full computation of  $M(J)$  for a particular state.

First, set up the state:

```
> s:=stateExample1(0.1,0.2,0.3,0.4);
```

Initialize the list of "known best channels" with 200 subintervals on the J axis.

```
> nticks:=200;
```

```
> minf:=Array(0..nticks-1);
```

```
  for i from 0 to nticks-1 do minf[i]:=Array([1,Array()]) end;
```

Try a number of randomly chosen channels.

```
> addSamples(s,10000,minf);
```

```
> plotResult(minf);
```

Refine the result by random variations, with a rather large standard deviation.

```
> refine(s,0.1,5,0.05,minf);
```

```
> plotResult(minf);
```

Refine with a smaller choice of standard variation.

```
> refine(s,0.05,10,0.05,minf);
```

```
> plotResult(minf);
```
